# Supplementary material for: FaCT: Faithful Concept Traces for Explaining Neural Network Decisions
Source: arXiv:2510.25512 source file (2026-04-13)
Supplement: Supplementary file 1 [file supp-qual-all-compressed.pdf]

# DenseNet-121 (Block 2/4)

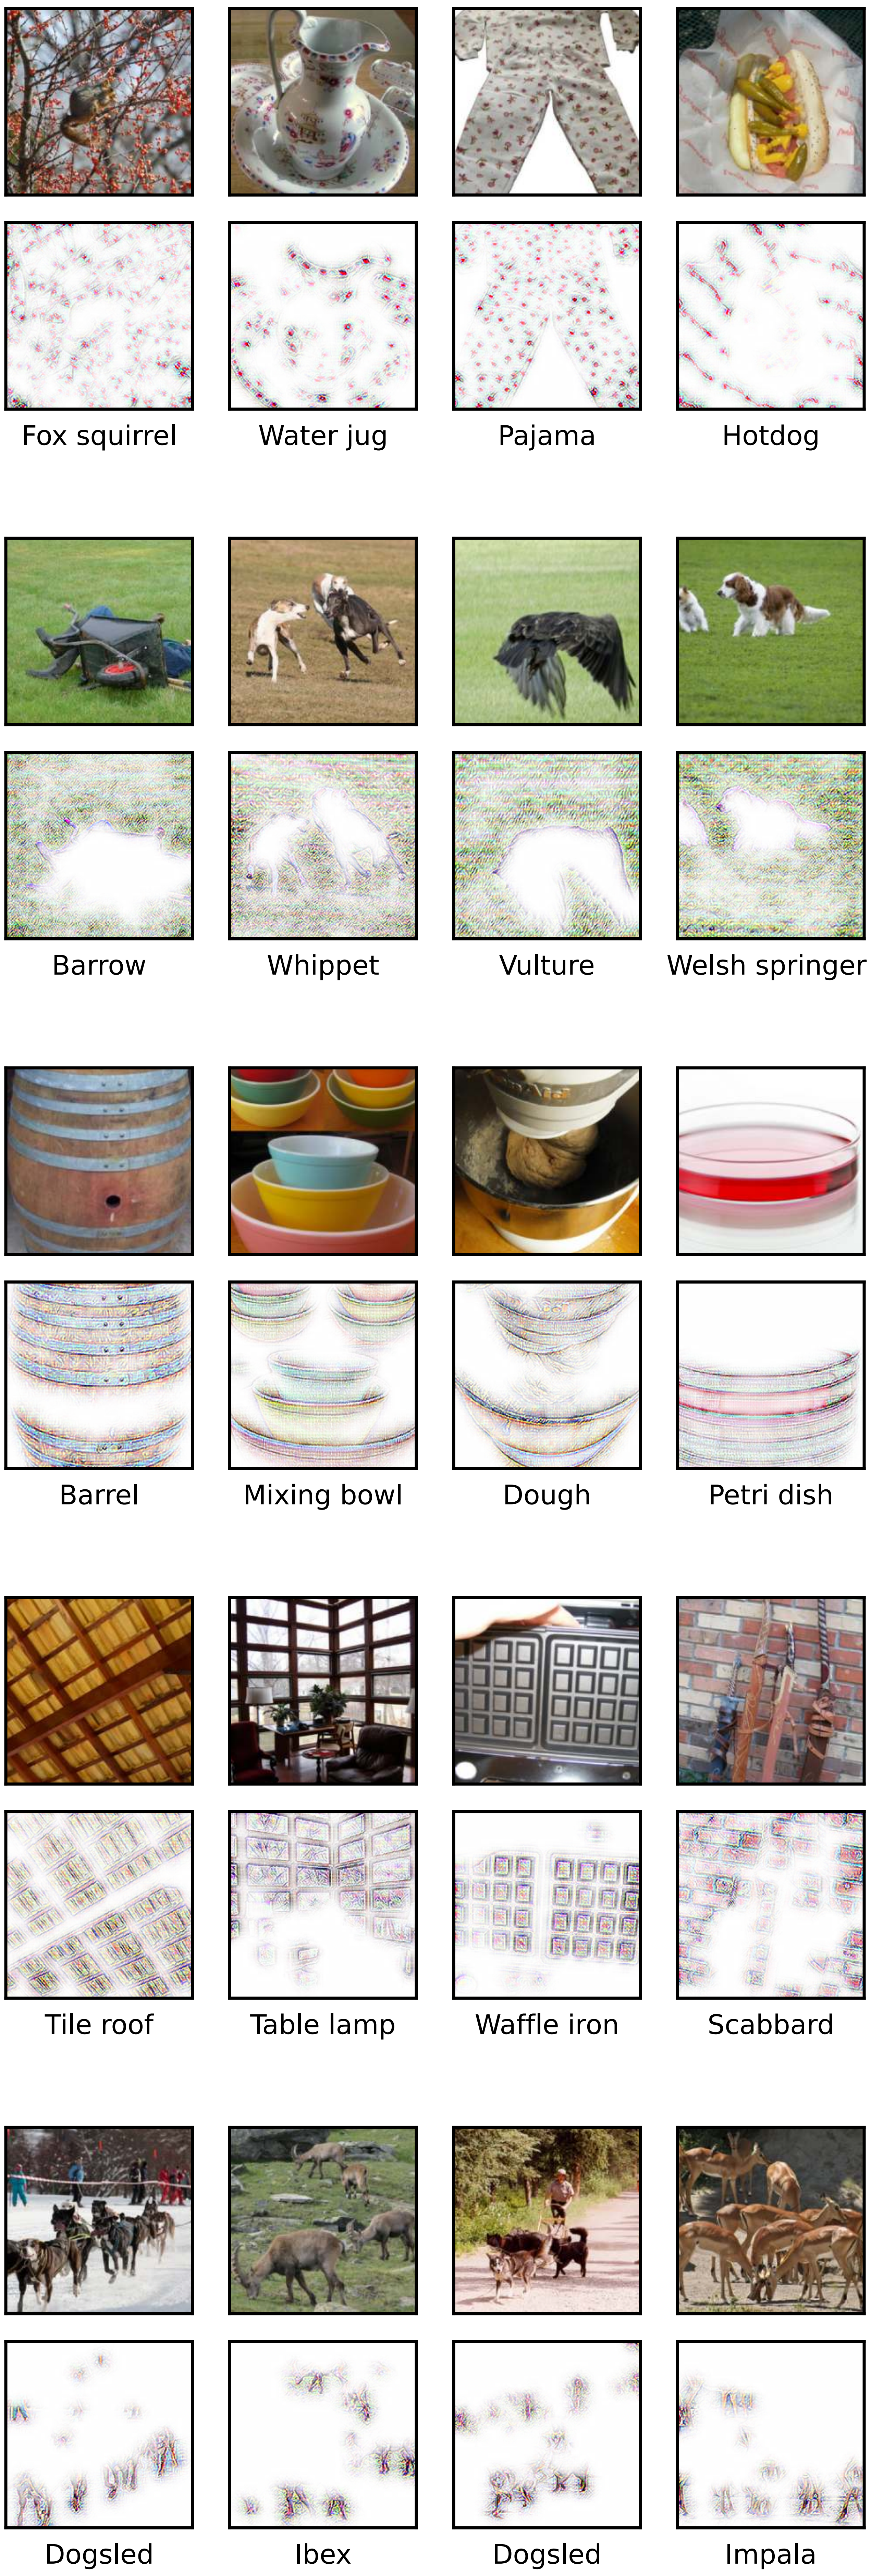

# DenseNet-121 (Block 4/4)

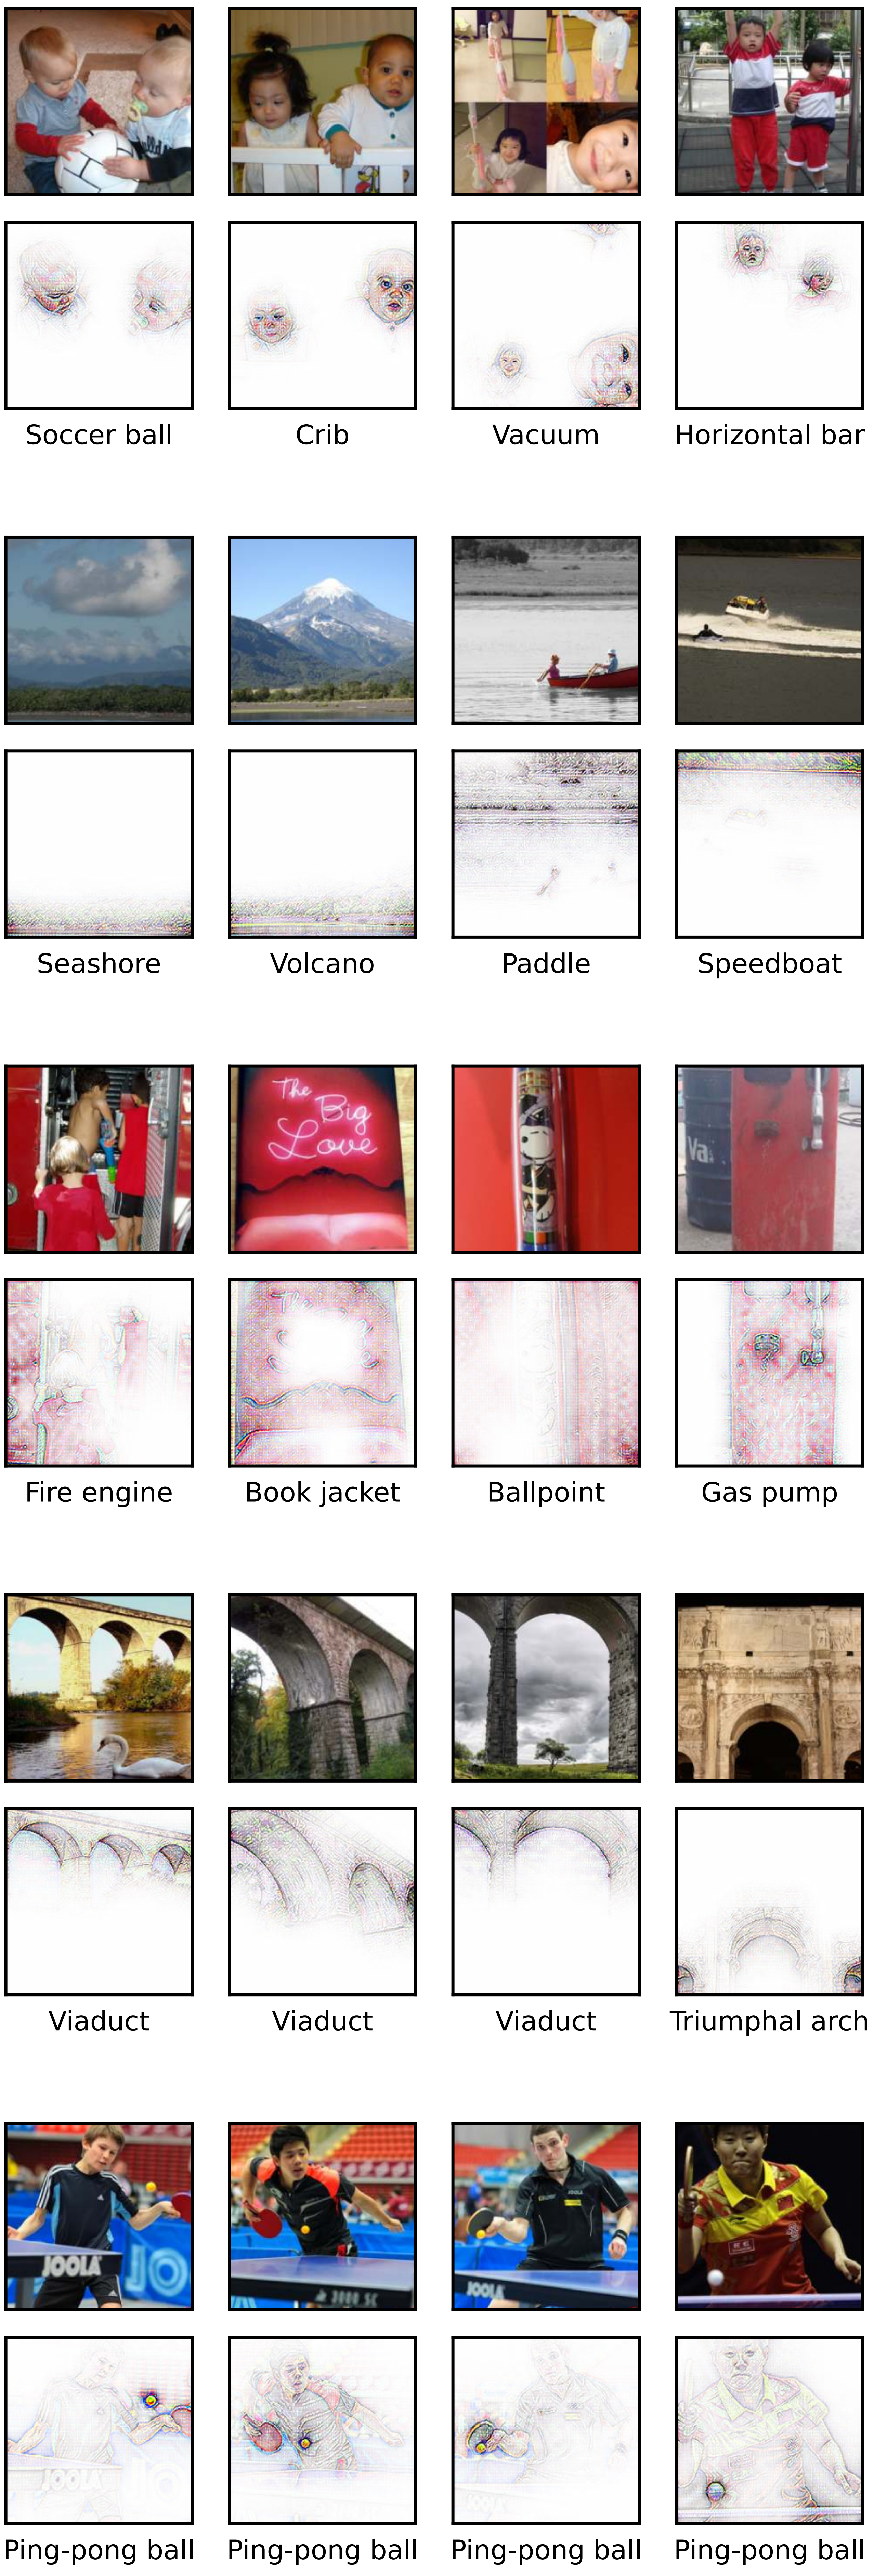

# $ViT_c$ - S (Block 9/10)

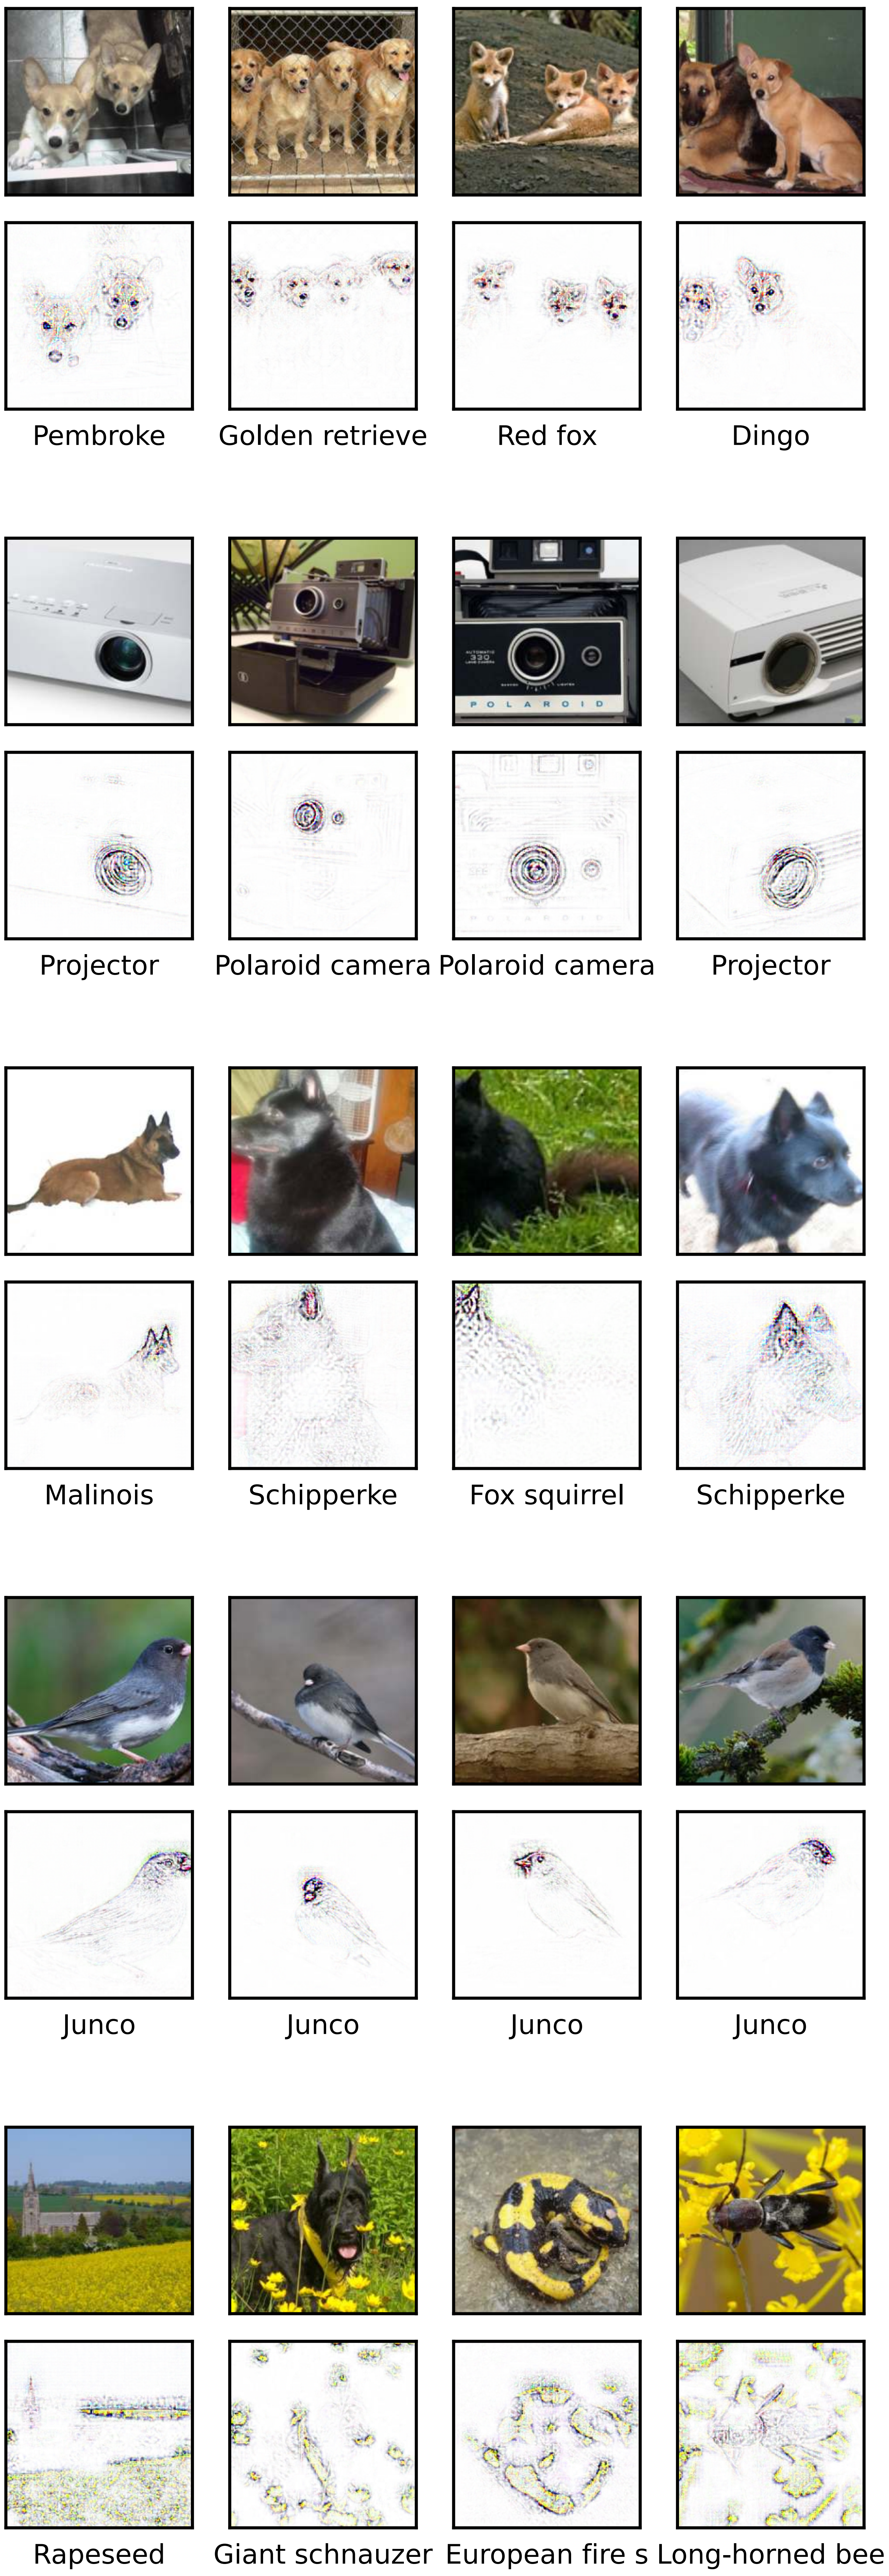

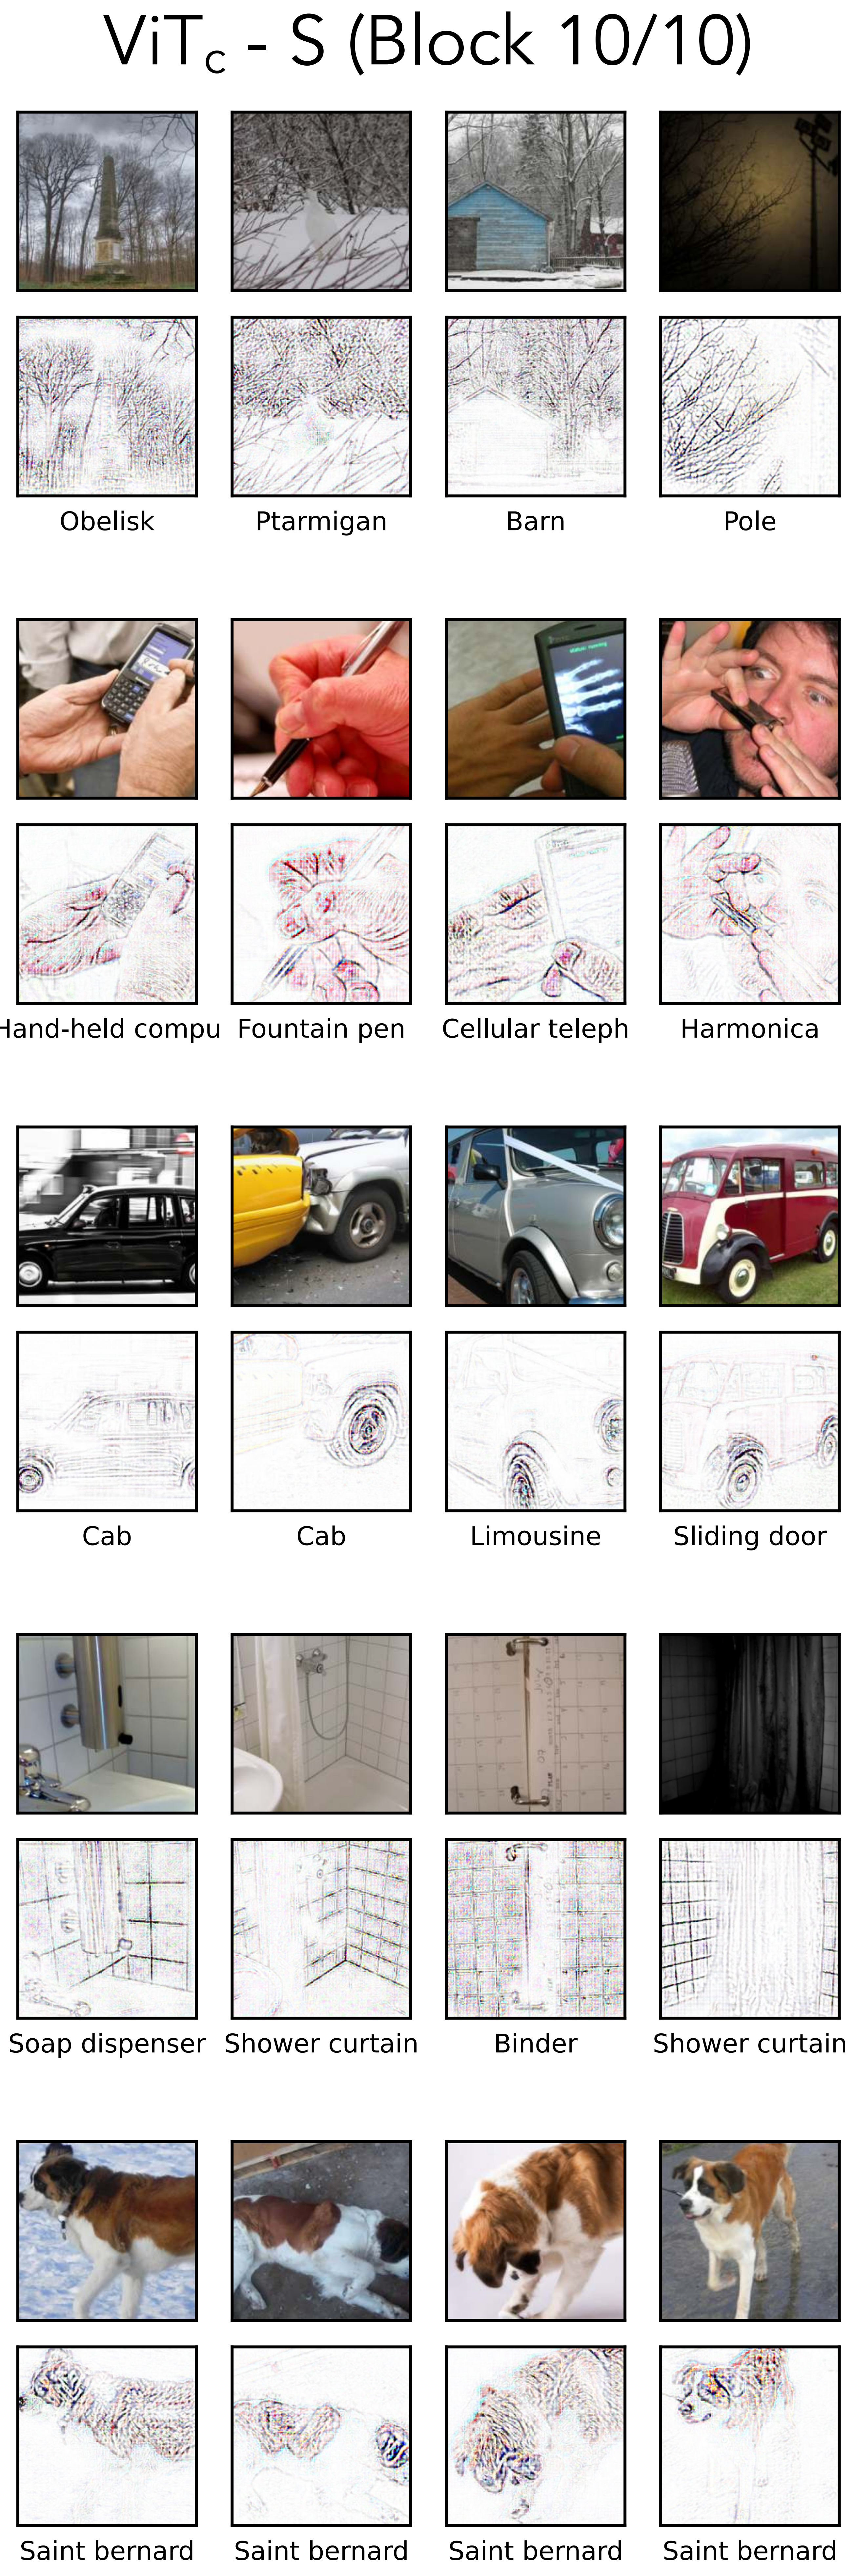
ViT$_c$ - S (Block 10/10)
Obelisk
Ptarmigan
Barn
Pole
Hand-held compu
Fountain pen
Cellular teleph
Harmonica
Cab
Cab
Limousine
Sliding door
Soap dispenser
Shower curtain
Binder
Shower curtain
Saint bernard
Saint bernard
Saint bernard
Saint bernard
